# Supplementary material for: Magnetism-induced band-edge shift as mechanism for magnetoconductance in CrPS$_4$ transistors
Source: arXiv:2304.12712 ancillary file (2023-08-21)
Supplement: Supplementary file 1 [file CPS4_MG.pdf]

# Magnetism-induced band-edge shift as mechanism for magnetoconductance in CrPS<sub>4</sub> transistors

Fan Wu,<sup>1,2,\*</sup> Marco Gibertini,<sup>3,4</sup> Kenji Watanabe,<sup>5</sup> Takashi Taniguchi,<sup>6</sup>  
Ignacio Gutiérrez-Lezama,<sup>1,2</sup> Nicolas Ubrig,<sup>1,2,†</sup> and Alberto F. Morpurgo<sup>1,2,‡</sup>

<sup>1</sup>*Department of Quantum Matter Physics, University of Geneva,  
24 Quai Ernest Ansermet, CH-1211 Geneva, Switzerland*

<sup>2</sup>*Department of Applied Physics, University of Geneva,  
24 Quai Ernest Ansermet, CH-1211 Geneva, Switzerland*

<sup>3</sup>*Dipartimento di Scienze Fisiche, Informatiche e Matematiche,  
University of Modena and Reggio Emilia, IT-41125 Modena, Italy*

<sup>4</sup>*Centro S3, CNR Istituto Nanoscienze, IT-41125 Modena, Italy*

<sup>5</sup>*Research Center for Functional Materials, National Institute  
for Materials Science, 1-1 Namiki, Tsukuba 305-0044, Japan*

<sup>6</sup>*International Center for Materials Nanoarchitectonics, National  
Institute for Materials Science, 1-1 Namiki, Tsukuba 305-0044, Japan*

## CONTENTS

|                                                                                                  |   |
|--------------------------------------------------------------------------------------------------|---|
| S1. Low temperature field-effect of CrPS <sub>4</sub> under magnetic field in additional devices | 2 |
| S2. Band structure calculations in different magnetic states                                     | 4 |
| S3. References                                                                                   | 6 |

---

\* fan.wu@unige.ch

† nicolas.ubrig@unige.ch

‡ alberto.morpurgo@unige.ch

## S1. LOW TEMPERATURE FIELD-EFFECT OF CrPS<sub>4</sub> UNDER MAGNETIC FIELD IN ADDITIONAL DEVICES

In the main text, we show that the large low-temperature magnetoconductance of CrPS<sub>4</sub> transistors originates from a magnetism-induced band-edge shift and we argue on the basis of data measured on a representative device. In the experiments, we have investigated in detail a total of three different devices, all of which show identical behavior. To demonstrate this device-to-device reproducibility, we show in Fig. S1 and Fig. S2 the conductance as a function of  $V_G$  at low temperature under different magnetic fields for the additional two devices (which we refer to as device S1 and S2, respectively).

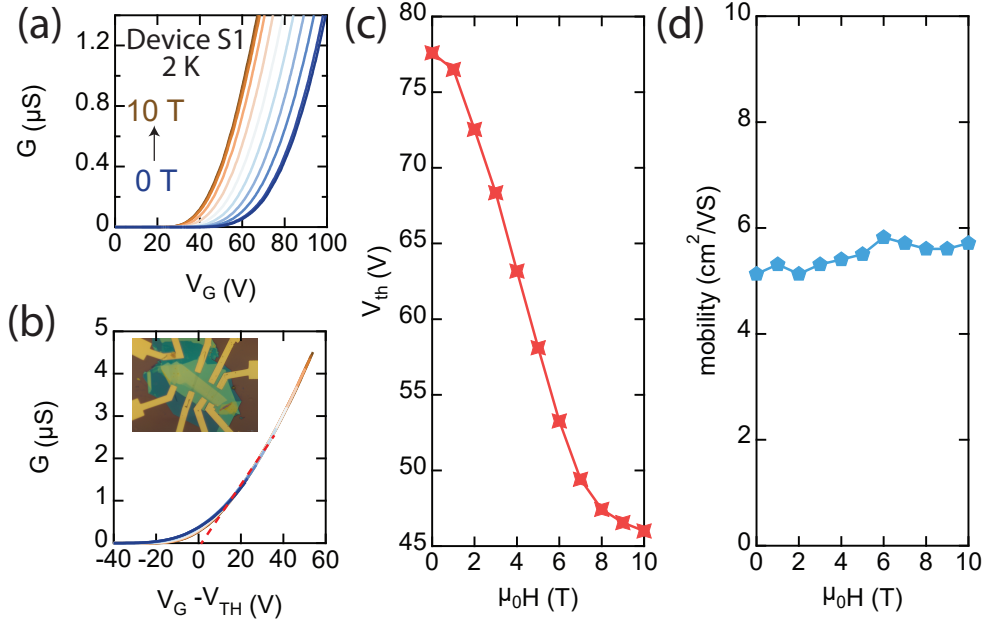

FIG. S1. Transfer curves of a transistor realized on a 9.7 nm CrPS<sub>4</sub> multilayer, measured at  $T = 2$  K for different values of magnetic field between 0 and 10 T. b) All transfer curves collapse, when plotted as a function of  $V_G - V_{TH}(H)$ . c) Threshold voltage and d) mobility at  $V_G = +100$  V, as determined from the transfer curves as a function of magnetic field. The shift in threshold voltage as magnetic field changes from 0 to 10 T and the magnetic state of the CrPS<sub>4</sub> multilayer changes is 31 V, in perfect agreement with the value found for the device discussed in the main text.

Fig. S1a shows the transfer curves of device S1 measured at  $T = 2$  K for different applied

magnetic fields. The thickness of the CrPS<sub>4</sub> multilayer is 9.7 nm. In analogy to the analysis in the main text, the transfer curves measured at different applied magnetic fields collapse when shifted by the respective threshold voltage,  $V_{\text{TH}}$ . In perfect agreement with the data presented in the main text, the dependence of the conductance on the field is due to the shift of  $V_{\text{TH}}$  with  $H$ , which quantitatively corresponds to the shift observed in the device in the main text ( $\Delta V_{\text{TH}} = 30$  V, see Fig. S1c). Also in complete agreement with the behavior discussed in the main text, the mobility is independent of  $H$ . Interestingly, even though the mobility of this device is significantly larger than the one in the main text (nearly 6 cm<sup>2</sup>/Vs versus 0.8 cm<sup>2</sup>/Vs for the device in the main text) the quantitative change in threshold voltage is identical in the two cases, indicating the robustness of the phenomenon.

Device S2 is about 10.7 nm thick and shows the same behavior as the others. In this device the gate voltage is applied by a graphite electrode placed under the bottom hBN layer used for encapsulation of the CrPS<sub>4</sub> multilayer. In this device, therefore, the gate dielectric is a 12 nm thick hBN crystal instead of 285 nm SiO<sub>2</sub> layer used in the device discussed in the main text and in device S1 here above. That is why in Fig. S2a the absolute gate voltage range is much narrower than in the other two devices (to compare the two type of devices,  $V_{\text{G}}$  needs to be normalized by the value of the capacitance to the gate electrode, see below). Figs. S2b-S2d (measurements taken at 0.3 K) confirm that also in this device  $V_{\text{TH}}$  shifts as a function of  $H$  and that the mobility  $\mu$  remains constant. By multiplying the threshold voltage shift by the capacitance to the gate, we obtain a change in carrier density of  $\Delta n = 2 \cdot 10^{12} \text{ cm}^{-2}$ , in excellent agreement with the value presented in the main text (*i.e.*, in excellent quantitative agreement with what we found in the device measured in the main text, as well as in device S1 here above).

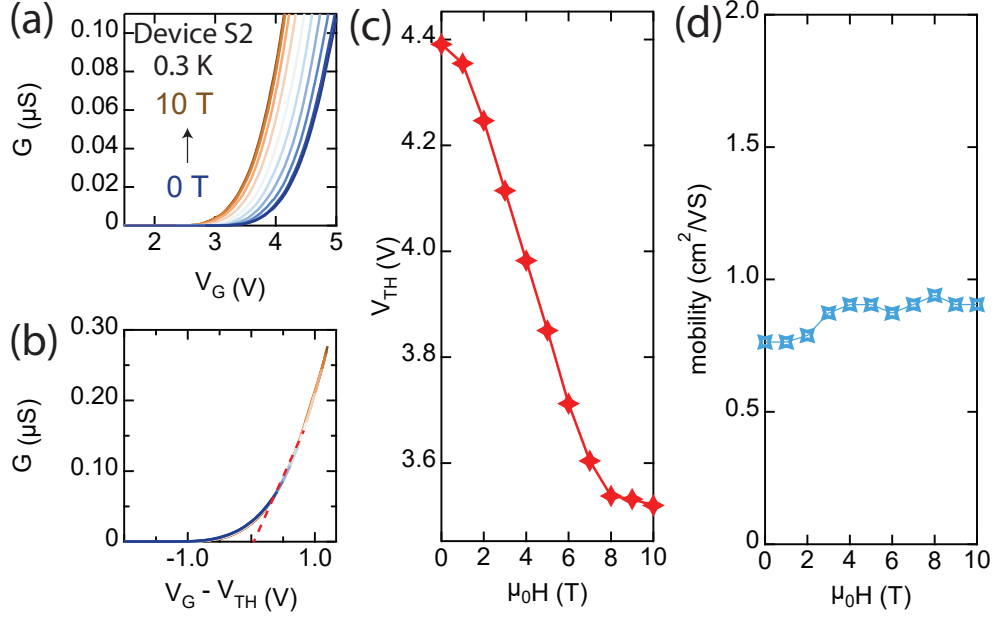

FIG. S2. Transfer curves of a transistor realized on a 10.7 nm thick CrPS<sub>4</sub> multilayer, measured at 0.3 K for different values of applied magnetic field between 0 and 10 T. In this device a bottom multilayer graphene strip acts as gate, separated from the CrPS<sub>4</sub> multilayer by a 12 nm thick h-BN crystal acting as gate dielectric. Because in this case the thickness of the gate dielectric is much smaller than that of the devices realized with 285 nm SiO<sub>2</sub> gate insulator, the corresponding gate capacitance is much larger, and the gate voltage that needs to be applied to induce conduction is correspondingly reduced. b) As for the other devices, when the data are plotted as a function of  $V_G - V_{TH}(H)$ , all transfer curves collapse on top of each other. c) Threshold voltage and d) mobility as determined from the transfer curves as a function of magnetic field. The threshold voltage has a shift of about 0.9 V, while the field effect mobility shows almost no change when the applied magnetic field changes from 0 to 10 T (antiferromagnetic to ferromagnetic ground state). When multiplied by the gate capacitance of the 12 nm h-BN gate insulator, the 0.9 V shift in threshold voltage corresponds to a shift in electron density of  $\Delta n \simeq 2 \cdot 10^{12} \text{ cm}^{-2}$ , in excellent agreement with what we observe in the devices with SiO<sub>2</sub> gate dielectric.

## S2. BAND STRUCTURE CALCULATIONS IN DIFFERENT MAGNETIC STATES

First-principles simulations were performed using the Quantum ESPRESSO distribution<sup>1,2</sup>. To account for van der Waals interactions between the layers, the spin-polarised extension<sup>3</sup> of the revised vdw-DF-cx exchange-correlation functional<sup>4,5</sup> was adopted, which



gives lattice parameters in good agreement with experiments. The Brillouin zone was sampled with a  $6 \times 6 \times 1$  ( $6 \times 6 \times 3$ )  $\Gamma$ -centered Monkhorst-Pack grid for multilayers (bulk). Pseudopotentials were taken from the Standard Solid-State Pseudopotential (SSSP) accuracy library (v1.0)<sup>6</sup> with cutoffs of 40 Ry and 320 Ry for wave functions and density, respectively. For multilayers, atomic positions and lattice parameters were extracted from the relaxed bulk crystal structure<sup>7</sup>, adding vacuum in the vertical direction and suppressing artificial interactions with spurious periodic replicas by using a Coulomb cutoff technique<sup>8</sup>. The band structure was computed along a high-symmetry path obtained by selecting the most interesting directions provided by SeekPath<sup>9</sup>.

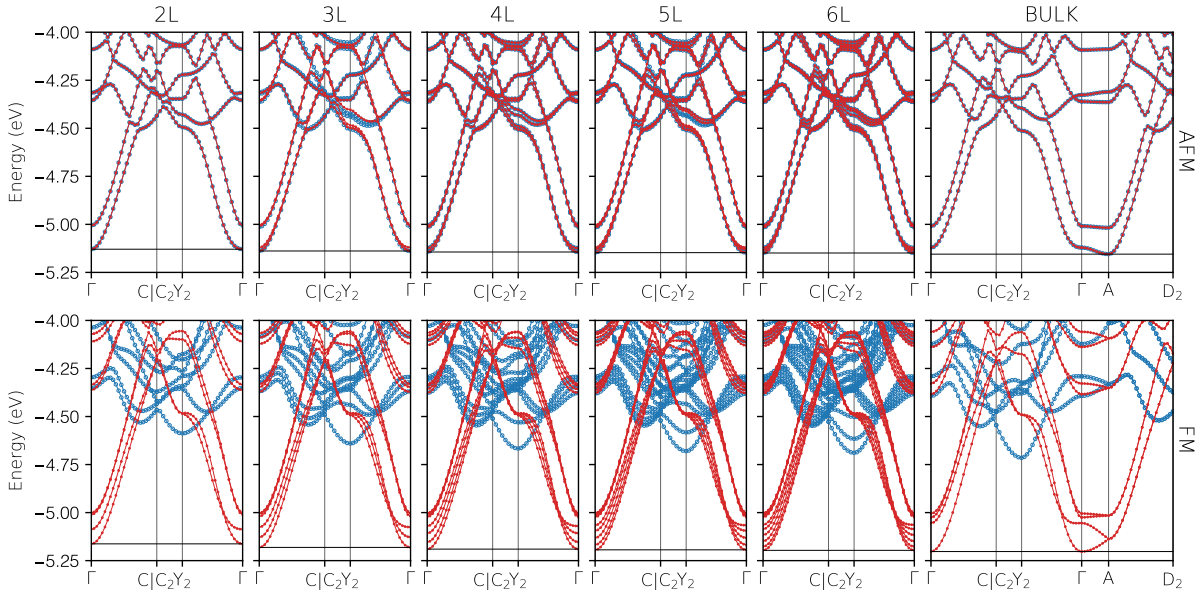

FIG. S3. Calculated band structure of  $\text{CrPS}_4$  multilayers and bulk in the antiferromagnetic (upper row) and ferromagnetic (lower row) states along a high-symmetry path in the Brillouin zone. Blue and red colors represent spin-up and spin-down states, respectively. For bulk  $\text{CrPS}_4$  the line  $\Gamma$  to A corresponds to the  $z$  direction orthogonal to the layers. The increase of bandwidth along this direction is responsible for the conduction to shift to lower energy when entering the ferromagnetic phase. In multilayers, the increase in bandwidth is reflected in a larger spread of the subbands arising from the lowest conduction band.

In the main text, we argued that the band-edge shift with the change of magnetic ordering from the antiferromagnetic to the ferromagnetic phase is mainly due to the enhancement of bandwidth along the perpendicular direction. In Fig. S3, we plot the results of first-

principles simulations of the band structure of CrPS<sub>4</sub> bulk and multilayers (for thicknesses ranging from 2 to 6) in both antiferromagnetic and ferromagnetic configurations. In all cases the simulations show that the total bandwidth of the conduction bands is larger in the ferromagnetic case than in the antiferromagnetic one, with a shift of the band-edge towards lower energies. In multilayers, this is associated with a larger spread of the subbands arising from the lowest conduction band, signalling a larger hybridization between the layers, *i.e.*, a larger hopping energy. In bulk, this is translated into an increase of the bandwidth along the *c*-direction (with also a shift of the conduction band minimum from A to  $\Gamma$ ). A simple analysis of the dispersion of the lowest conduction band along this direction shows that it can be interpreted in terms of a simple tight-binding model where hopping between nearest layers is suppressed in the antiferromagnetic configuration, while it is allowed in the ferromagnetic one, resulting in the larger bandwidth. The shift in the band-edge increases with thickness, ranging from 33 meV for the bilayer to 48 meV in the hexalayer, which is essentially indistinguishable from the bulk value obtained by aligning the deep semicore states of Chromium.

### S3. REFERENCES

- [1] P. Giannozzi, S. Baroni, N. Bonini, M. Calandra, R. Car, C. Cavazzoni, Davide Ceresoli, G. L. Chiarotti, M. Cococcioni, I. Dabo, A. D. Corso, S. d. Gironcoli, S. Fabris, G. Fratesi, R. Gebauer, U. Gerstmann, C. Gougoussis, Anton Kokalj, M. Lazzeri, L. Martin-Samos, N. Marzari, F. Mauri, R. Mazzarello, Stefano Paolini, A. Pasquarello, L. Paulatto, C. Sbraccia, S. Scandolo, G. Sclauzero, A. P. Seitsonen, A. Smogunov, P. Umari, and R. M. Wentzcovitch, *Journal of Physics: Condensed Matter* **21**, 395502 (2009).
- [2] P. Giannozzi, O. Andreussi, T. Brumme, O. Bunau, M. Buongiorno Nardelli, M. Calandra, R. Car, C. Cavazzoni, D. Ceresoli, M. Cococcioni, N. Colonna, I. Carnimeo, A. Dal Corso, S. De Gironcoli, P. Delugas, R. A. Distasio, A. Ferretti, A. Floris, G. Fratesi, G. Fugallo, R. Gebauer, U. Gerstmann, F. Giustino, T. Gorni, J. Jia, M. Kawamura, H. Y. Ko, A. Kokalj, E. Küçükbenli, M. Lazzeri, M. Marsili, N. Marzari, F. Mauri, N. L. Nguyen, H. V. Nguyen, A. Otero-De-La-Roza, L. Paulatto, S. Poncé, D. Rocca, R. Sabatini, B. Santra, M. Schlipf, A. P. Seitsonen, A. Smogunov, I. Timrov, T. Thonhauser, P. Umari, N. Vast, X. Wu, and

- S. Baroni, Journal of Physics Condensed Matter **29**, 465901 (2017).
- [3] T. Thonhauser, S. Zuluaga, C. Arter, K. Berland, E. Schröder, and P. Hyldgaard, Physical Review Letters **115**, 136402 (2015).
- [4] M. Dion, H. Rydberg, E. Schroder, D. C. Langreth, and B. I. Lundqvist, Physical Review Letters **92**, 246401 (2004).
- [5] K. Lee, E. D. Murray, L. Kong, B. I. Lundqvist, and D. C. Langreth, Physical Review B **82**, 081101 (2010).
- [6] G. Prandini, A. Marrazzo, I. E. Castelli, N. Mounet, and N. Marzari, npj Computational Materials **4**, 72 (2018).
- [7] F. Wu, M. Gibertini, K. Watanabe, T. Taniguchi, I. Gutiérrez-Lezama, N. Ubrig, and A. F. Morpurgo, Advanced Materials **35**, 2211653 (2023).
- [8] T. Sohler, M. Calandra, and F. Mauri, Phys. Rev. B **96**, 075448 (2017).
- [9] Y. Hinuma, G. Pizzi, Y. Kumagai, F. Oba, and I. Tanaka, Computational Materials Science **128**, 140 (2017).
